# Supplementary material for: Action of $w_0$ on $V^L$: the special case of $\mathfrak{so}(1,n)$
Source: arXiv:2310.14956 ancillary file (2023-10-23)
Supplement: Supplementary file 1 [file readme.pdf]

## Implementation of the algorithm in LiE

The files given here contain an implementation of the algorithm in the LiE software package. The package, and information about it, can be found here: <http://www.mathlabo.univ-poitiers.fr/~maavl/LiE/>.

### Quick description

The LiE code in the files `lie_code_type_An.txt`, `lie_code_type_Bn.txt` etc. defines, for most simple real Lie algebras  $\mathfrak{g}_{\mathbb{R}}$  of low rank, a function called `w0`/*name of  $\mathfrak{g}_{\mathbb{R}}$* / with the following specifications:

- Input: an integral dominant weight  $\lambda$  of  $\mathfrak{g} = \mathfrak{g}_{\mathbb{R}}^{\mathbb{C}}$  (i.e. an element of  $Q \cap \mathfrak{h}^+$ ), specified by its coordinates (which are nonnegative integers) in the basis formed by the fundamental weights, listed in the Bourbaki order.
- Output: the  $w_0$ -signature of the representation  $V_{\lambda}$  of  $\mathfrak{g}$ , i.e. the signature of the linear involution  $w_0|_{V_{\lambda}^I}$  (see [LFS18, Def. 1.2]; the bibliography can be found in the main article).

These functions all rely on an underlying function called `count_signature`, which is defined in the file `lie_code_common.txt`.

### How to compute the $w_0$ -action

As an example, suppose that we want to compute the action of  $w_0$  on  $V_{\lambda}^I$  for  $\mathfrak{g}_{\mathbb{R}} = \mathfrak{su}(1, 3)$ , and  $\lambda = 4\varpi_1 + 3\varpi_2 + 2\varpi_3$  (which is  $(5, 1, -2, -4)$  in the  $\varepsilon_i$  basis). We then start by executing in LiE all of the code from `lie_code_common.txt`. We then execute the code that defines the function `w0SU3_1`, which we find in the file `lie_code_type_An.txt`:

```
> resSU3_1 = res_mat([[1,0,0],
>                     [0,0,1]], A3)
> w0SU3_1(vec v) = count_signature(branch(v,A1A1T1,resSU3_1,A3),[-2,0,0])
```

We then call that function on the desired highest weight, and LiE gives us the  $w_0$ -signature:

```
> w0SU3_1([4,3,2])
[1,2]
```

This tells us that in this case, the linear involution  $w_0|_{V_{\lambda}^I}$  has eigenvalue 1 with multiplicity 1 and eigenvalue  $-1$  with multiplicity 2.

### How to write the algebra-specific code

Now what if we want to work with some algebra  $\mathfrak{g}_{\mathbb{R}}$  that does not have its code already written? Then we can define the corresponding restriction matrix `res`/*name of  $\mathfrak{g}_{\mathbb{R}}$* / and then signature function `w0`/*name of  $\mathfrak{g}_{\mathbb{R}}$* /, by using the following blueprint:

`res[name of  $\mathfrak{g}_{\mathbb{R}}$ ] = res_mat([roots of  $\mathfrak{s}$ ], [type of  $\mathfrak{g}$ ])`  
`w0[name of  $\mathfrak{g}_{\mathbb{R}}$ ] = count_signature(branch(v, [type of  $\mathfrak{s}$ ], res[name of  $\mathfrak{g}_{\mathbb{R}}$ ], [type of  $\mathfrak{g}$ ]), [mask]),`

where:

- *[name of  $\mathfrak{g}_{\mathbb{R}}$ ]* can be whatever character string chosen by the user to represent the group  $\mathfrak{g}_{\mathbb{R}}$  (LiE has no predefined names for real forms).
- *[type of  $\mathfrak{g}$ ]* (resp. *[type of  $\mathfrak{s}$ ]*) is the type of  $\mathfrak{g} = \mathfrak{g}_{\mathbb{R}}^{\mathbb{C}}$  (resp. of  $\mathfrak{s} = \mathfrak{s}_{\mathbb{R}}^{\mathbb{C}}$ ), with the abelian part designated by the letter T and necessarily put at the end. For example, A12B2T3 stands for  $A_{12} \oplus B_2 \oplus \mathbb{C}^3$ , i.e.  $\mathfrak{sl}_{13}(\mathbb{C}) \oplus \mathfrak{so}_5(\mathbb{C}) \oplus \mathbb{C}^3$ .
- *[roots of  $\mathfrak{s}$ ]* is the list of the simple roots of  $\mathfrak{s}$ , which can be read off Table 2 in the appendix of the article. These roots must be expressed in the basis formed by the simple roots of  $\mathfrak{g}$  (for exceptional algebras, this is already how they are presented in the table). They must be listed in the Bourbaki order within each factor, concatenated together in the order in which the factors of *[type of  $\mathfrak{s}$ ]* are written.
- *[mask]* is a tuple of integers that depends on the type of  $\mathfrak{s}_{\mathbb{R}}$  as a *real* algebra. The mask of each individual factor can be looked up in Table 1 below; they are then, once again, concatenated together in the order in which the factors of *[type of  $\mathfrak{s}$ ]* are written.

## How the code works

Let us start with the common part of the code (i.e. the file `lie_code_common.txt`). It defines two functions: `tot_sign` and `count_signature`.

The goal of the function `tot_sign` is essentially to compute the action of  $w_0$  on the subspace  $V_{\lambda}^{l(\mathfrak{s}_{\mathbb{R}})}$  of some single irreducible representation  $V_{\lambda}$  (with highest weight  $\lambda$ ) of  $\mathfrak{s}_{\mathbb{R}}$ . By construction, this subspace then has dimension at most 1, so the action of  $w_0$  is either  $\pm \text{Id}$  or 0. The specific sign can be computed by the formula given in the third column of Table 1 below, which is a conversion of the formula given in Lemma 2.1 of the article, from the  $(\varepsilon_1, \dots, \varepsilon_n)$  basis (which is convenient to minimize case distinctions) to the  $(\varpi_1, \dots, \varpi_r)$  basis (in which LiE works).

We see that most of the time, the sign is obtained as a product of some functions  $\xi_k^{\sigma}$  of the individual coordinates. These functions  $\xi_k^{\sigma} : \mathbb{Z}^{\geq 0} \rightarrow \{-1, 0, 1\}$  are defined, for each  $k \in \mathbb{Z}^{\geq 0}$  and  $\sigma = \pm 1$ , by

$$\xi_k^{\sigma}(n) := \begin{cases} \sigma^{\frac{n}{k}} & \text{if } n \in k\mathbb{Z}; \\ 0 & \text{otherwise,} \end{cases}$$

with the convention  $\xi_0^+(0) = 1$ . We then encode the coefficients of these functions in the “mask” passed as a parameter to `tot_sign`, with  $\pm k$  standing for  $\xi_k^{\pm}$ . There is however a slight deviation from this pattern for  $\mathfrak{so}(1, 5)$ , which we encode by the “magical”

Table 1: Formula for the  $w_0$ -sign in each factor of  $\mathfrak{s}_{\mathbb{R}}$ , and its encoding as a “mask”.

| Factor $\mathfrak{s}_{\mathbb{R},i}$ of $\mathfrak{s}_{\mathbb{R}}$ | Type of its complexification | Sign of $w_0 _{V_{\lambda}^{l(\mathfrak{s}_{\mathbb{R}},i)}}$ ,<br>for $\lambda = c_1\varpi_1 + \dots + c_k\varpi_k$ . | Corresponding mask |
|---------------------------------------------------------------------|------------------------------|------------------------------------------------------------------------------------------------------------------------|--------------------|
| $\mathfrak{so}(1, 2)$                                               | A1                           | $\xi_2^-(c_1)$                                                                                                         | [-2]               |
| $\mathfrak{so}(1, 3)$                                               | A1A1                         | $\xi_2^-(c_1)\xi_2^-(c_2)$                                                                                             | [-2, -2]           |
| $\mathfrak{so}(1, 4)$                                               | B2                           | $\xi_2^+(c_1)\xi_2^-(c_2)$                                                                                             | [2, -2]            |
| $\mathfrak{so}(1, 5)$                                               | D3                           | $\xi_2^+(c_1)\xi_1^-(c_2 + c_3)\xi_0^+(c_2 - c_3)$                                                                     | [2, 51, -1]        |
| $\mathfrak{so}(1, 2k), k \geq 3$                                    | Bk                           | $\xi_2^+(c_1)\xi_1^-(c_2)\xi_0^+(c_3) \dots \xi_0^+(c_k)$                                                              | [2, -1, 0, ..., 0] |
| $\mathfrak{so}(1, 2k - 1), k \geq 4$                                | Dk                           | $\xi_2^+(c_1)\xi_1^-(c_2)\xi_0^+(c_3) \dots \xi_0^+(c_k)$                                                              | [2, -1, 0, ..., 0] |
| any compact factor                                                  | various                      | $\xi_0^+(c_1) \dots \xi_0^+(c_k)$                                                                                      | [0, ..., 0]        |
| $\mathbb{R}^k$                                                      | Tk                           | $\xi_0^+(c_1) \dots \xi_0^+(c_k)$                                                                                      | [0, ..., 0]        |

placeholder value 51. (Of course it would have been cleaner to use a type other than **int** for this placeholder value, but LiE does not support tuples of mixed type!)

As for the function **count\_signature**, it simply takes as input:

- a “polynomial” in the terminology of LiE, which is essentially a tuple of weights, representing the direct sum of the irreducible representations of  $\mathfrak{s}$  having these weights;
- and a mask,

and tallies up the **tot\_sign** values of all the summands computed with the given mask, as a signature  $(p, q)$  where  $p$  and  $q$  represent the respective multiplicity of +1 and -1.

Now each of the functions **w0/name of  $\mathfrak{g}_{\mathbb{R}}$**  simply decomposes a representation of  $\mathfrak{g}$  into irreducible representations of  $\mathfrak{s}$  (using the **branch** routine provided by LiE), and then calls **count\_signature** to compute the  $w_0$ -signature of that restricted representation, which we know to be equal to the  $w_0$ -signature of the original representation thanks to Theorem 3.1 of the article.
